# Supplementary material for: Self-Consistent Description of Vapor-Liquid Interface in Ionic Fluids
Source: arXiv:2206.02030 ancillary file (2022-10-12)
Supplement: Supplementary file 1 [file Supp__info_Interface_letter.pdf]

# Supplemental Material for

## Self-Consistent Description of Vapor-Liquid Interface in Ionic Fluids

Nikhil R. Agrawal<sup>1</sup> and Rui Wang<sup>1,2,\*</sup>

<sup>1</sup>*Department of Chemical and Biomolecular Engineering,  
University of California, Berkeley, California 94720, USA*

<sup>2</sup>*Materials Sciences Division, Lawrence Berkeley National Laboratory, Berkeley, 94720, California, USA*

### I. DERIVATION OF THE GENERAL THEORY

The derivation begins by writing the electrostatic Hamiltonian,  $\mathcal{H}$ . For an electrolyte solution containing a salt with ions of valency  $q_{\pm}$ ,  $\mathcal{H}$  for the system can be written as

$$\mathcal{H} = \frac{e^2}{2} \int d\mathbf{r} d\mathbf{r}' \rho(\mathbf{r}) C(\mathbf{r}, \mathbf{r}') \rho(\mathbf{r}') \quad (1)$$

where  $\rho(\mathbf{r})$  is the total charge density at position  $\mathbf{r}$

$$e\rho(\mathbf{r}) = e\rho_{ex}(\mathbf{r}) + e \int d\mathbf{r}' [q_+ h_+(\mathbf{r} - \mathbf{r}') \hat{c}_+(\mathbf{r}') - q_- h_-(\mathbf{r} - \mathbf{r}') \hat{c}_-(\mathbf{r}')] \quad (2)$$

$C$  is the Coulomb operator

$$-\nabla \cdot [\epsilon(\mathbf{r}) \nabla C(\mathbf{r}, \mathbf{r}')] = \delta(\mathbf{r} - \mathbf{r}') \quad (3)$$

$\hat{c}_{\pm,s}(\mathbf{r}) = \sum_{i,s} \delta(\mathbf{r} - \mathbf{r}_i)$  is the particle density operator for the ion or solvent  $s$ , the function  $h_{\pm}(\mathbf{r} - \mathbf{r}')$  is the charge distribution function for the ion centered at  $\mathbf{r}'$ ,  $e$  is elementary charge, and  $\epsilon(\mathbf{r}) = kT\epsilon_0\epsilon(\mathbf{r})/e^2$  is the scaled permittivity with  $\epsilon_0$  the vacuum permittivity.

Using  $\mathcal{H}$ , the grand canonical partition function,  $\Xi$ , could be written as shown in Equation 4, where  $\mu$ ,  $n$ , and  $v$  denote chemical potential, number, and molecular volume of the ions and solvent, respectively.

$$\Xi = \sum_{n_+, -, s=0}^{\infty} \frac{e^{\mu_+ n_+} e^{\mu_s n_s} e^{\mu_s n_s}}{n_+! n_-! n_s! v_+^{n_+} v_-^{n_-} v_s^{n_s}} \int \prod_{i=1}^{n_+} d\mathbf{r}_i \prod_{j=1}^{n_-} d\mathbf{r}_j \prod_{k=1}^{n_s} d\mathbf{r}_k \times \prod_{\mathbf{r}} \delta(1 - \hat{c}_+(\mathbf{r})v_+ - \hat{c}_-(\mathbf{r})v_- - \hat{c}_s(\mathbf{r})v_s) \exp(-\beta\mathcal{H}) \quad (4)$$

The functional delta is added to include the excluded volume effect of the ions and solvent. We then perform the usual Hubbard-Stratonovich transformation (HST) and Fourier transformation (FT) to change the particle variables to field variables. HST introduces a field variable for potential,  $\phi(\mathbf{r})$ , coupled with  $\rho(\mathbf{r})$ , and FT when applied on the functional delta introduces a field variable  $\xi(\mathbf{r})$  for the incompressibility condition.

$$\Xi = \frac{1}{Z_0} \int D\phi \int D\xi \exp[-L[\phi, \xi]], \text{ where} \quad (5)$$

$$Z_0 = \int D\phi \exp \left[ -\frac{1}{2} \int d\mathbf{r} \epsilon (\nabla \phi)^2 \right] \text{ and } L = \int d\mathbf{r} \left[ \frac{1}{2} \epsilon (\nabla \phi)^2 + i\rho_{ex}\phi - \sum_{j=+,-} \lambda_j e^{-iq_j \int d\mathbf{r}' h_j(\mathbf{r}-\mathbf{r}') \phi(\mathbf{r}') - iv_j \xi} - \lambda_s e^{-iv_s \xi} - i\xi \right]$$

where  $\lambda_{j,s} = \frac{e^{\mu_{j,s}}}{v_{j,s}}$  is the fugacity. The integration over  $\xi(\mathbf{r})$  is then approximated using saddle point method, which yields the following expression in terms of  $\xi(\mathbf{r})$ 's saddle point value  $-i\eta(\mathbf{r})$ ,

$$v_+ \lambda_+ e^{-iq_+ \hat{h}_+ \phi - v_+ \eta} + v_- \lambda_- e^{iq_- \hat{h}_- \phi - v_- \eta} + v_s \lambda_s e^{-v_s \eta} - 1 = 0 \quad (6)$$

---

\* email: [ruiwang325@berkeley.edu](mailto:ruiwang325@berkeley.edu)

where we have used short-hand notation  $\hat{h}_\pm \phi$  for local spatial averaging of  $\phi$  by the charge distribution function:  $\hat{h}_\pm \phi = \int d\mathbf{r}' h_\pm(\mathbf{r}' - \mathbf{r}) \phi(\mathbf{r}')$ . This partition function can now be simplified to

$$\Xi = \frac{1}{Z_0} \int D\phi \exp \left\{ - \int d\mathbf{r} \left[ \frac{1}{2} \epsilon (\nabla \phi)^2 + i \rho_{ex} \phi - \lambda_+ e^{-iq_+ \hat{h}_+ \phi - v_+ \eta} - \lambda_- e^{iq_- \hat{h}_- \phi - v_- \eta} - \lambda_s e^{-v_s \eta} - \eta \right] \right\} \quad (7)$$

Next to estimate the integral in  $\phi$  a variational calculation for the grand free energy  $\mathcal{W}$  is done using the Gibbs-Feynman-Bogoliubov (GFB) bound. To calculate the bound we took the reference action to be of the Gaussian form centered around the mean potential,  $-i\psi$ .

$$\mathcal{W}(-\mathcal{L}[\phi]) = -\ln \Xi \leq -\ln \Xi_{ref} + \langle \mathcal{L}[\phi] - \mathcal{L}_{ref}[\phi] \rangle_{ref} \quad (8)$$

$$\mathcal{L}_{ref} = \frac{1}{2} \int d\mathbf{r} d\mathbf{r}' [\phi(\mathbf{r}) + i\psi(\mathbf{r})] G(\mathbf{r}, \mathbf{r}') [\phi(\mathbf{r}') + i\psi(\mathbf{r}')] \quad (9)$$

Using the above Gaussian reference action and mathematical manipulations similar to the ones given in [1–3], the variational free energy turns out to be

$$\begin{aligned} \mathcal{W}_{var} = -\ln \Xi = & -\frac{1}{2} \ln \left[ \frac{\det G}{\det C} \right] - \frac{1}{2} \int d\mathbf{r} d\mathbf{r}' [\det G^{-1}(\mathbf{r}, \mathbf{r}') - \det C^{-1}(\mathbf{r}, \mathbf{r}')] G(\mathbf{r}, \mathbf{r}') - \frac{1}{2} \int d\mathbf{r} [\epsilon(\mathbf{r}) (\nabla \psi(\mathbf{r}))^2] \\ & - \int d\mathbf{r} [\lambda_+ e^{-q_+ \psi - u_+ - v_+ \eta} + \lambda_- e^{q_- \psi - u_- - v_- \eta} + \lambda_s e^{-v_s \eta} + \eta - \rho_{ex} \psi] \end{aligned} \quad (10)$$

$$u_\pm(\mathbf{r}) = \frac{q_\pm^2}{2} \int d\mathbf{r}' d\mathbf{r}'' h_\pm(\mathbf{r} - \mathbf{r}') G(\mathbf{r}', \mathbf{r}'') h_\pm(\mathbf{r}'' - \mathbf{r}) \quad (11)$$

where  $u_+$  is the self energy of ions (Equation 11), and  $G$  is the correlation function corresponding to the reference action. Minimizing  $\mathcal{W}$  with respect to  $G$  and  $\psi$  give us the following set of self consistent equations

$$-\nabla_{\mathbf{r}} \cdot [\epsilon(\mathbf{r}) \nabla_{\mathbf{r}} G(\mathbf{r}, \mathbf{r}')] + 2I(\mathbf{r}) G(\mathbf{r}, \mathbf{r}') = \delta(\mathbf{r} - \mathbf{r}') \quad (12)$$

$$-\nabla \cdot [\epsilon(\mathbf{r}) \nabla \psi(\mathbf{r})] = \rho_{ex}(\mathbf{r}) + q_+ c_+(\mathbf{r}) - q_- c_-(\mathbf{r}) \quad (13)$$

$$c_\pm(\mathbf{r}) = \lambda_\pm \exp[-q_\pm \psi(\mathbf{r}) - u_\pm(\mathbf{r}) - v_\pm \eta(\mathbf{r})] \quad (14)$$

$$c_s(\mathbf{r}) = \lambda_s \exp[-v_s \eta(\mathbf{r})] \quad (15)$$

where  $2I(\mathbf{r}) = \epsilon(\mathbf{r}) \kappa^2(\mathbf{r}) = c_+(\mathbf{r}) q_+^2 + c_-(\mathbf{r}) q_-^2$  is the local ionic strength. In physical terms,  $G(\mathbf{r}, \mathbf{r}')$  is the conditional potential at  $\mathbf{r}$  generated by a point charge at  $\mathbf{r}'$  mediated by other mobile ions in the presence of spatially varying dielectric constant and ionic strength. An expression for  $\eta(\mathbf{r})$  in terms of bulk concentrations of ions and chemical potential of solvent can be derived by combining Eq. 15 with the following incompressibility constraint

$$v_+ c_+(\mathbf{r}) + v_- c_-(\mathbf{r}) + v_s c_s(\mathbf{r}) = 1 \quad (16)$$

With the help of above equations and using the charging method to simplify the free energy expression given in Equation 10, the following expression for minimised grand free energy is derived

$$\begin{aligned} W = \int d\mathbf{r} \left[ \frac{1}{2} \psi (\rho_{ex} - q_+ c_+ + q_- c_-) - c_+ - c_- - c_s - \eta \right] & + \frac{1}{2} \int d\mathbf{r} \int d\mathbf{r}' \int d\mathbf{r}'' \int_0^1 d\tau [G(\mathbf{r}', \mathbf{r}'', \tau) - G(\mathbf{r}', \mathbf{r}'')] \\ & \times \left[ \sum_{j=+, -} q_j^2 c_j h_j(\mathbf{r}' - \mathbf{r}) h_j(\mathbf{r} - \mathbf{r}'') \right] \end{aligned} \quad (17)$$

where  $\tau$  is the ‘charging’ variable.

## II. BULK THERMODYNAMICS

As explained in the main text, for a Gaussian distribution of charge over the ion given by

$$h_{\pm}(\mathbf{r} - \mathbf{r}') = \left( \frac{1}{2a_{\pm}} \right)^{3/2} \exp \left[ \frac{-\pi(\mathbf{r} - \mathbf{r}')^2}{2a_{\pm}^2} \right] \quad (18)$$

the self-energy in the bulk  $u_{\pm,b}$  is

$$u_{\pm,b} = \frac{q_{\pm}^2}{8\pi\epsilon} \left[ \frac{1}{a_{\pm}} - \kappa_b \exp \left( \frac{(a_{\pm}\kappa_b)^2}{\pi} \right) \operatorname{erfc} \left( \frac{a_{\pm}\kappa_b}{\sqrt{\pi}} \right) \right] \quad (19)$$

where  $a_i$  is the radius of the ion associated with volume  $v_i$ . By combining Eqs. 14, 15 and 24 following expressions for chemical potentials can be written

$$\mu_{\pm} = \mp q_{\pm} \psi_b + u_{\pm,b} + \ln c_{\pm,b} v_{\pm} + v_{\pm} \eta_b \quad (20)$$

$$\mu_s = \ln c_{s,b} v_s + v_s \eta_b \quad (21)$$

From Eq. 17 we get an expression for bulk pressure

$$P_b = c_{+,b} + c_{-,b} + c_{s,b} + \eta_b - \frac{1}{2} \int d\mathbf{r}' \int d\mathbf{r}'' \int_0^1 d\tau [G_b(\mathbf{r}', \mathbf{r}'', \tau) - G_b(\mathbf{r}', \mathbf{r}'')] \left[ \sum_{j=+,-} q_j^2 c_{j,b} h_j(\mathbf{r}' - \mathbf{r}) h_j(\mathbf{r} - \mathbf{r}'') \right] \quad (22)$$

Using the above equations for bulk chemical potentials and pressures written as an explicit function of bulk concentration and electrostatic potentials we can calculate the two-phase co-existence curve. In case of asymmetric electrolytes, these equations should give us a non-zero value of Galvani potential,  $\Delta\psi_G$ . Here without loss of generality, we have taken the potential of vapor phase to be zero and the potential of liquid phase to be  $\psi_G$ .

## III. INTERFACIAL BEHAVIOR

The self-energy in the interface is given by

$$u_{\pm}(\mathbf{r}) = u_{\pm,s}(\mathbf{r}) + \frac{q_{\pm}^2}{2} G_l(\mathbf{r}, \mathbf{r}) \quad (23)$$

where  $u_{\pm,s}(\mathbf{r})$  is

$$u_{\pm,s}(\mathbf{r}) = \frac{q_{\pm}^2}{8\pi\epsilon(\mathbf{r})} \left[ \frac{1}{a_{\pm}} - \kappa(\mathbf{r}) \exp \left( \frac{(a_{\pm}\kappa(\mathbf{r}))^2}{\pi} \right) \operatorname{erfc} \left( \frac{a_{\pm}\kappa(\mathbf{r})}{\sqrt{\pi}} \right) \right] \quad (24)$$

and the differential equation for  $G_l$  is

$$-\nabla_{\mathbf{r}'} \cdot [\epsilon(\mathbf{r}') \nabla_{\mathbf{r}'} G_l(\mathbf{r}', \mathbf{r}'')] + 2I(\mathbf{r}') G_l(\mathbf{r}', \mathbf{r}'') = S(\mathbf{r}', \mathbf{r}'') \quad (25)$$

where the non-local source term  $S$  is

$$S(\mathbf{r}', \mathbf{r}'') = \nabla_{\mathbf{r}'} \cdot (\epsilon(\mathbf{r}') - \epsilon(\mathbf{r}'')) \nabla_{\mathbf{r}'} G_s(\mathbf{r}', \mathbf{r}'') - 2(I(\mathbf{r}') - I(\mathbf{r}'')) G_s(\mathbf{r}', \mathbf{r}'')$$

Since for the planar vapor-liquid interface problem there is symmetry in  $x - y$  directions parallel to the interface we first write  $G_l$  in cylindrical coordinates  $(r, \theta, z)$  and then apply Fourier transform in  $r$  and  $\theta$  directions using the following definition

$$G_l(r, z', z'') = \int_0^\infty \frac{J_0(sr)}{2\pi} \hat{G}_l(s, z', z'') s ds \quad (26)$$

where  $J_0$  is the zeroth order Bessel function. The Fourier transformed version of Equation 25 is

$$-\frac{\partial}{\partial z'} [\epsilon(z') \frac{\partial \hat{G}_l(s, z', z'')}{\partial z'}] + \epsilon(z') (\kappa^2(z') + s^2) \hat{G}_l(s, z', z'') = \hat{S}(s, z', z'')$$

where  $\hat{S}$  is

$$\hat{S}(s, z', z'') = \frac{\partial}{\partial z'} [(\epsilon(z') - \epsilon(z'')) \frac{\partial \hat{G}_s(s, z', z'')}{\partial z'}] - (\epsilon(z')(\kappa^2(z') + s^2) - \epsilon(z'')(\kappa^2(z'') + s^2)) \hat{G}_s(s, z', z'') \quad (27)$$

An analytical solution for  $\hat{G}_s$  exists and is given by

$$\hat{G}_s(s, z', z'') = \frac{e^{-p|z' - z''|}}{2p\epsilon(z'')}, \text{ where } p = (s^2 + \kappa^2(z''))^{1/2} \quad (28)$$

Equation 27 and 28 can be solved using a finite difference scheme to calculate the self energy. However, in this work we have used the following alternative route to solve for  $G_l$ , a well established process which has been used in previous works as well[4, 5]. In this other route, we start by rewriting equation for  $u_{\pm}(\mathbf{r})$  using the functions  $G$  and  $G_s$  as shown below

$$u_{\pm}(\mathbf{r}) = u_{\pm,s}(\mathbf{r}) + \frac{q_{\pm}^2}{2} \lim_{\mathbf{r}', \mathbf{r}'' \rightarrow \mathbf{r}} (G(\mathbf{r}', \mathbf{r}'') - G_s(\mathbf{r}', \mathbf{r}'')) \quad (29)$$

The above equation can be further simplified by using the free space correlation function  $G_o(\mathbf{r}', \mathbf{r}'')$  (Equation 30) defined using local  $\epsilon(\mathbf{r})$ , Equation 29 can now be rewritten as 31

$$-\epsilon(\mathbf{r}) \nabla_{\mathbf{r}'}^2 G_o(\mathbf{r}', \mathbf{r}'') = \delta(\mathbf{r}', \mathbf{r}'') \quad (30)$$

$$u_{\pm}(\mathbf{r}) = u_{\pm,s}(\mathbf{r}) + \frac{q_{\pm}^2}{2} \lim_{\mathbf{r}', \mathbf{r}'' \rightarrow \mathbf{r}} (G - G_o) + \frac{q_{\pm}^2}{2} \lim_{\mathbf{r}', \mathbf{r}'' \rightarrow \mathbf{r}} (G_o - G_s) \quad (31)$$

Careful evaluation of the limit in the third term gives

$$u_{\pm}(\mathbf{r}) = u_{\pm,s}(\mathbf{r}) + \frac{q_{\pm}^2 \kappa(\mathbf{r})}{8\pi\epsilon(\mathbf{r})} + \frac{q_{\pm}^2}{2} \lim_{\mathbf{r}', \mathbf{r}'' \rightarrow \mathbf{r}} (G - G_o) \quad (32)$$

Similar to  $G_l$  we can also use Fourier transform to solve for  $G$  and  $G_o$ . The Fourier transformed versions of Eq. 12 and 30 are

$$-\frac{\partial}{\partial z'} [\epsilon(z') \frac{\partial \hat{G}(s, z', z'')}{\partial z'}] + \epsilon(z')(\kappa^2(z') + s^2) \hat{G}(s, z', z'') = \delta(z', z'') \quad (33)$$

$$-\frac{\partial^2 \hat{G}_o(s, z', z'')}{\partial z'^2} + s^2 \hat{G}_o(s, z', z'') = \frac{\delta(z', z'')}{\epsilon(z)} \quad (34)$$

The limit term of Eq. 32 can be written in terms of  $\hat{G}$  and  $\hat{G}_o$  as

$$\frac{q_{\pm}^2}{2} \lim_{\mathbf{r}', \mathbf{r}'' \rightarrow \mathbf{r}} (G - G_o) = \frac{q_{\pm}^2}{4\pi} \int_0^\infty (\hat{G}(s, z, z) - \hat{G}_o(s, z, z)) s ds \quad (35)$$

Equations till this point are very general and are applicable for any symmetric planar interface with spatially varying ionic strength or dielectric function. The boundary conditions (BCs) shown next are for the case of primitive model with constant  $\epsilon$ , a case which has been solved for in the current work. For the solution domain  $z' \in [0, L]$ , vapor phase is placed in the region  $z' < 0$  and liquid phase in the region  $z' > L$ . The BCs for  $\hat{G}$  are

$$\frac{\partial \hat{G}(s, z', z'')}{\partial z'} = (s^2 + \kappa_v^2)^{1/2} \hat{G}(s, z', z'') \quad (36)$$

$$\frac{\partial \hat{G}(s, z', z'')}{\partial z'} = -(s^2 + \kappa_l^2)^{1/2} \hat{G}(s, z', z'') \quad (37)$$

which are applicable for  $z' < 0, z'' \geq 0$  and  $z' > L, z'' \leq L$  respectively. Here  $\kappa_v$  and  $\kappa_l$  are the bulk screening constant in vapor and liquid phase, respectively. These BCs are derived using continuity of  $\hat{G}$  and its first derivative at the ends. The boundary conditions for  $\hat{G}_o$  are similar with the only difference being that  $\kappa_v$  and  $\kappa_l$  are replaced by 0. Only other BCs needed are for  $\psi$  which are  $\psi(z' = 0) = 0$  and  $\psi(z' = L) = \psi_G$ .

- 
- [1] R. R. Netz and H. Orland, *Eur. Phys. J. E* **11**, 301 (2003).
  - [2] Z. G. Wang, *Physical Review E - Statistical, Nonlinear, and Soft Matter Physics* **81**, 021501 (2010).
  - [3] N. Agrawal and R. Wang [10.48550/arxiv.2205.14222](https://arxiv.org/abs/2205.14222) (2022).
  - [4] R. Wang and Z. G. Wang, *Journal of Chemical Physics* **144**, 134902 (2016).
  - [5] Z. Xu and A. C. Maggs, *Journal of Computational Physics* **275**, 310 (2014).
